# Supplementary material for: PROTECT: Protein circadian time prediction using unsupervised learning
Source: arXiv:2501.07405 source file (2025-01-13)
Supplement: Supplementary file 1 [file supp.pdf]

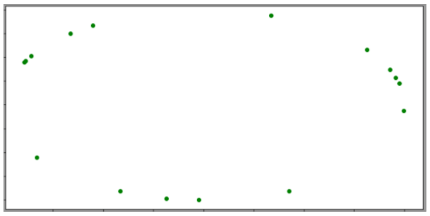

Figure S1: Mouse liver encoded data in pre-training stage.

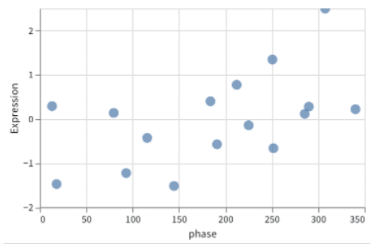


(a) First epoch

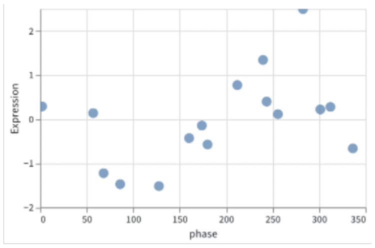


(b) Last epoch

Figure S2: Training progress on a random protein in mouse liver data during fine-tuning stage.

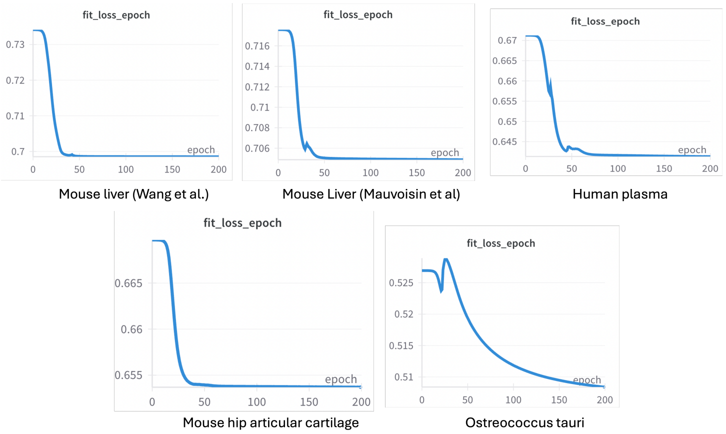


Figure S3: Convergence results on time labeled datasets.

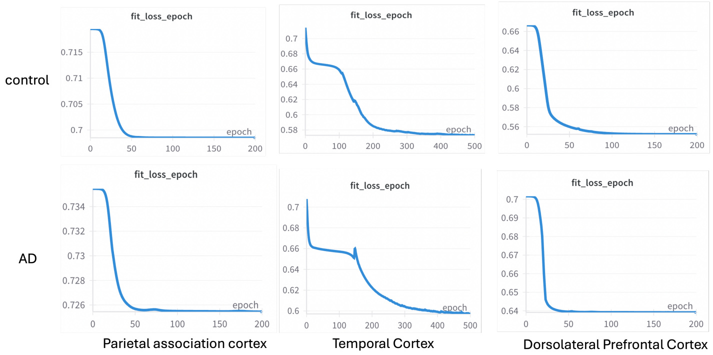


Figure S4: Convergence results on brain datasets.

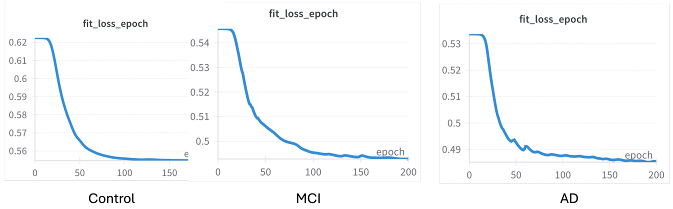


Figure S5: Convergence results on urine dataset.

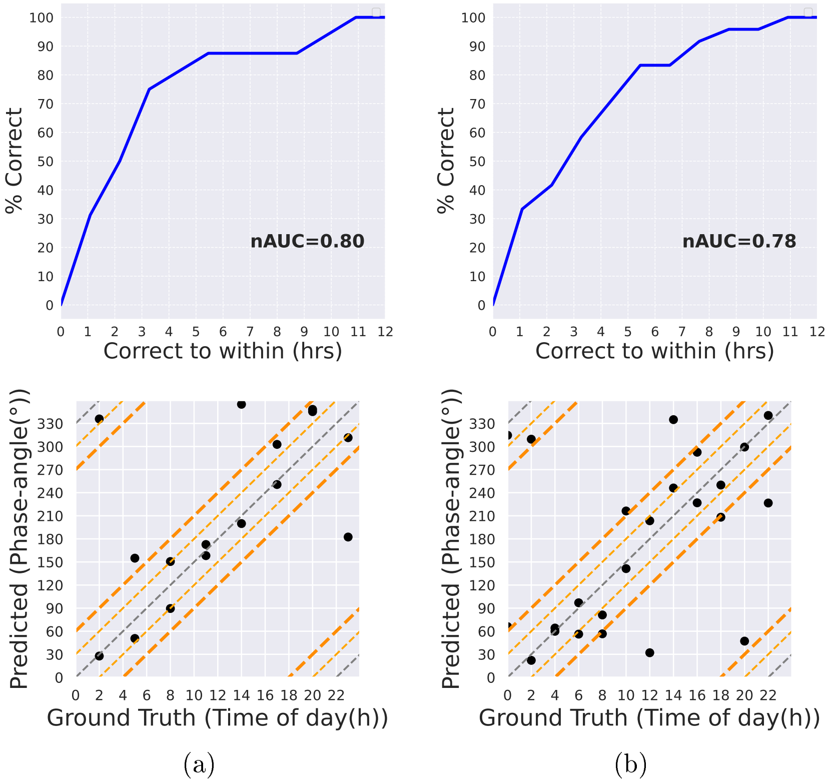


Figure S6: Accuracy of PROTECT on (a) mouse liver and (b) mouse BAT tissues. The top row shows ROC curves where the y-axis shows the fraction of correctly predicted samples, and the x-axis shows the size of errors. The bottom row shows the scatter plots of predictions vs ground truth.

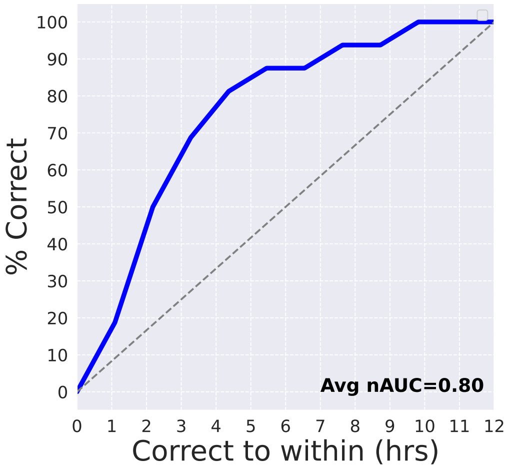


**(a)**

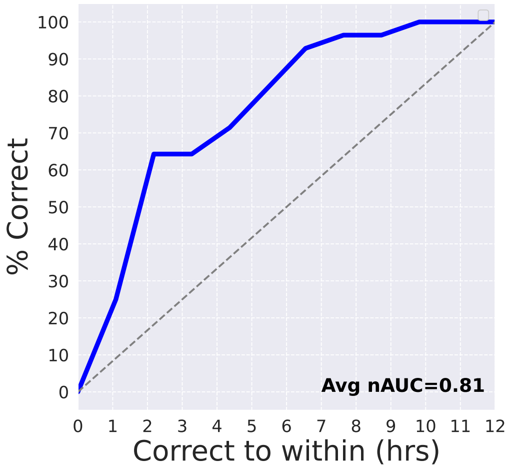


**(b)**

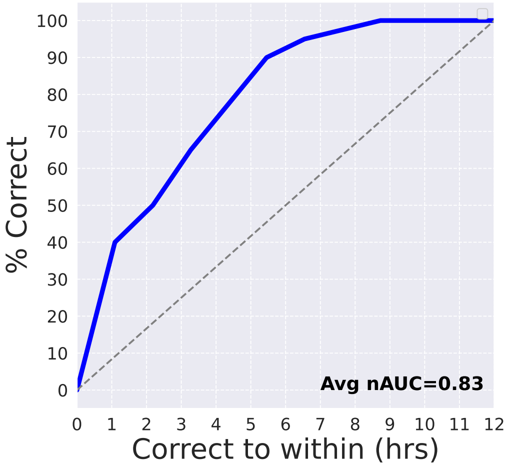


**(c)**

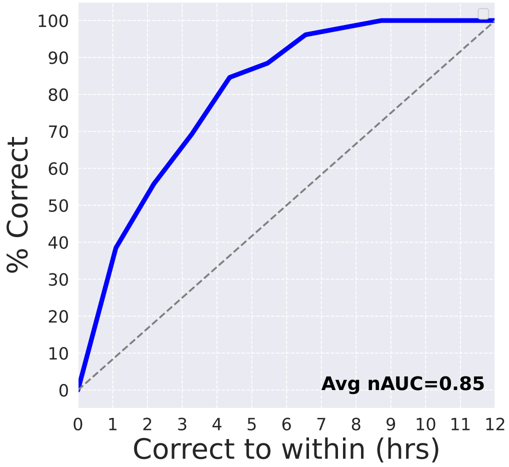


**(d)**

Figure S7: Results on mouse liver dataset of Wang et al. [34] using less number of samples: (a) using 4 samples, (b) using 7 samples, (c) using 10 samples, and (d) using 13 samples.

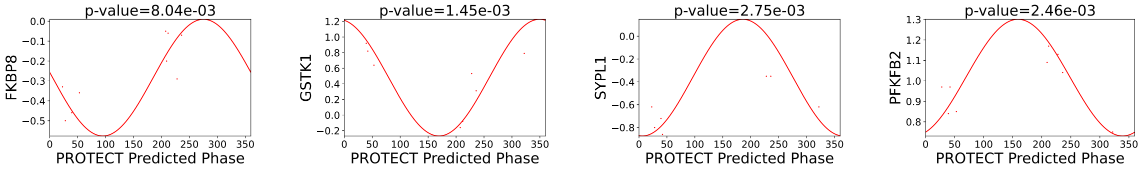


Figure S8: Plots of four randomly chosen proteins known to be rhythmic in thyroid tissue using predicted phases by PROTECT. The y-axis represents protein expression levels, and the x-axis represents the predicted phases (in degrees) as determined by PROTECT.

Table S1: Intersection of rhythmic proteins in 3 brain regions

| **Intersection Group** | **Number of Proteins** |
|---|---|
| All 3 Control Sets | 276 |
| All 3 AD sets | 271 |
| Control $\ominus$ AD | 4 |
| AD $\ominus$ Control | 0 |

| **DLFPC Region** | **Parital Association Cortex Region** | **Urine** |
|---|---|---|
| SEPT11 | ANLN | SERPINA7 |
| CTNNB1 | HIP1 | KRT7 |
| TARDBP | LIPS | HLA-A |
| AAK1 | MBP | CRNN |
| TSNAX | SIR2 | EVPL |
| CORO1A | CN37 | MPO |
| DNAJA3 | MYO1D | TUBB3 |
| PCLO | CD9 | C9 |
| PIGN | DOCK1 | KRT75 |
| PPP1R7 | HSPA1L | ANXA3 |
| FGA | CRNKL1 | SERPINA1 |
| SDHA | HSPD1 | SERPINA3 |
| FGG | SHROOM4 | YWHAZ |
| VDAC1 | CA14 | A1BG |
| ACTN2 | FMNL2 | KRT79 |
| ACTR2 | MYO1E | FGG |
| NCAM2 | ADA10 | HPX |
| SEPT9 | GAPR1 | SERPIND1 |
| F13A1 | DAAM2 | HSP90AB1 |
| PLCL1 | CSPG2 | GATM |

Table S2: First 20 Hub Proteins in DLFPC, parital association cortex, and urine datasets

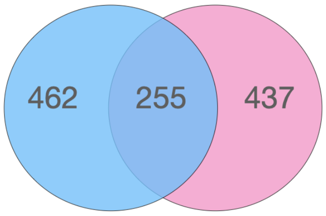


(a)

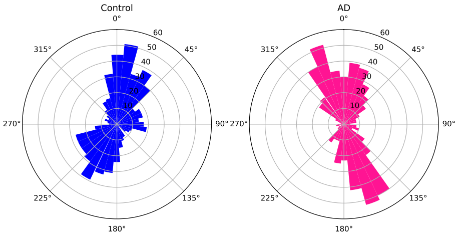


(b)

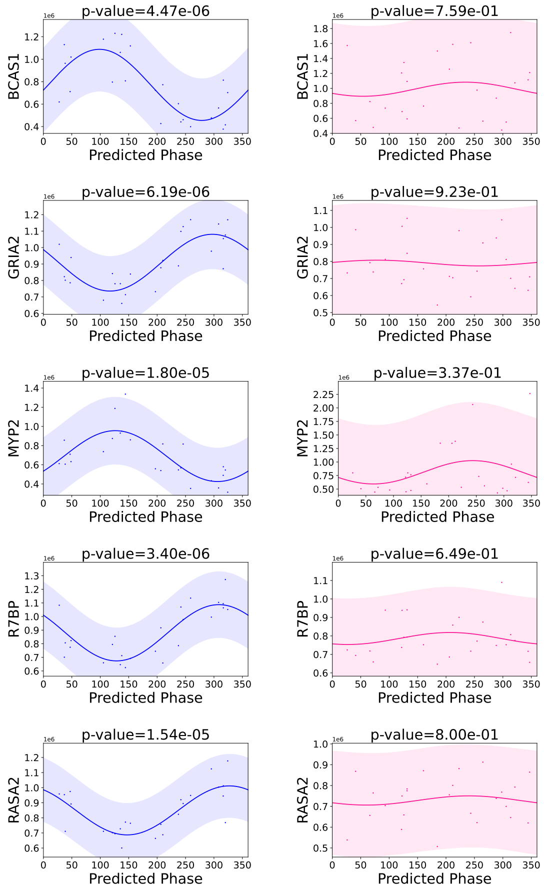


(c)

Figure S9: Disparities between control and AD subjects in parietal association cortex using PROTECT predicted phases. (a) Venn diagram of numbers of rhythmic proteins in control (blue) and AD (pink) subjects. (b) Rose plots of distributions of peak times (i.e., acrophases) in rhythmic proteins of control and AD subjects within 24 hours (360 degrees) of the circadian cycle. The radial distance indicates protein counts. (c) Plots of 5 example rhythmic proteins in control subjects that lose rhythmicity in AD.

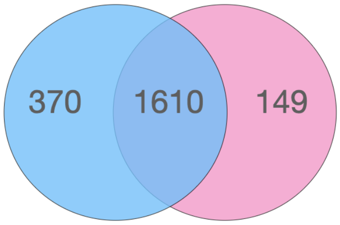


(a)

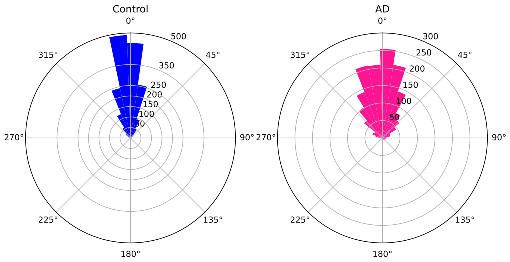


(b)

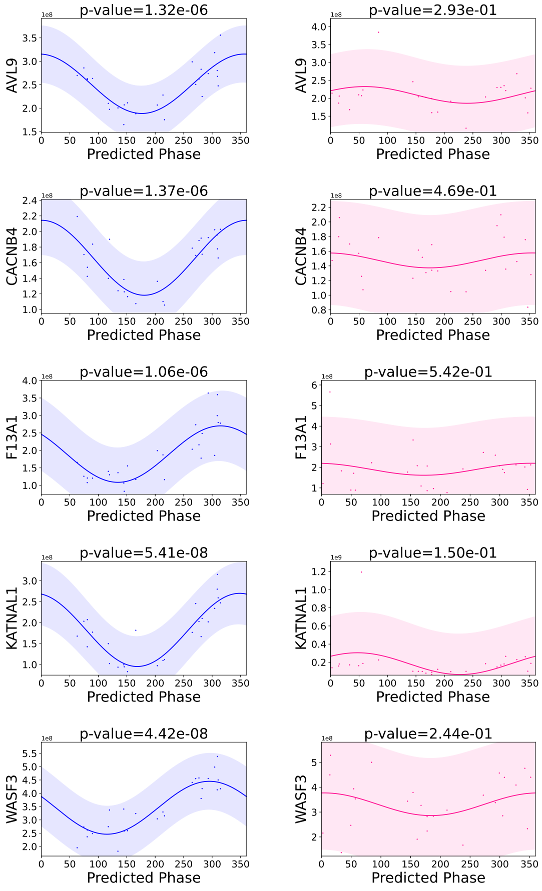


(c)

Figure S10: Disparities between control and AD subjects in DLFPC using PROTECT predicted phases. (a) Venn diagram of numbers of rhythmic proteins in control (blue) and AD (pink) subjects. (b) Rose plots of distributions of peak times (i.e., acrophases) in rhythmic proteins of control and AD subjects within 24 hours (360 degrees) of the circadian cycle. The radial distance indicates protein counts. It is noted that the max of radial distance differs between control and AD plots. (c) Plots of 5 example rhythmic proteins in control subjects that lose rhythmicity in AD.

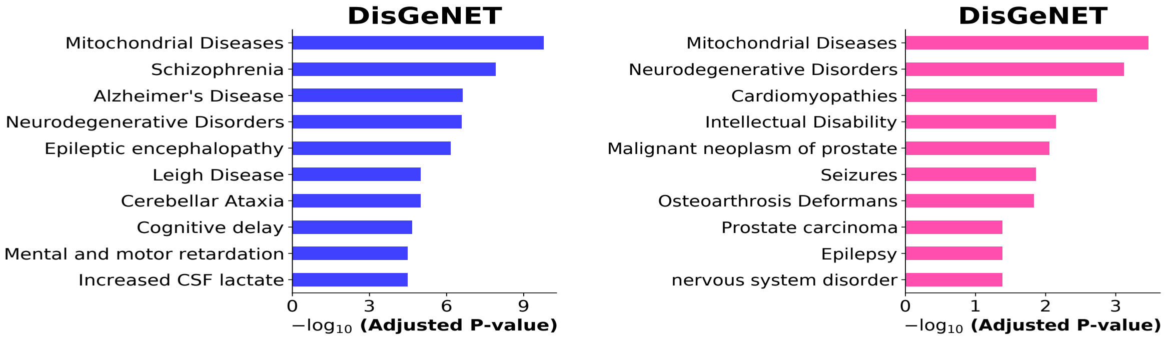


(a)

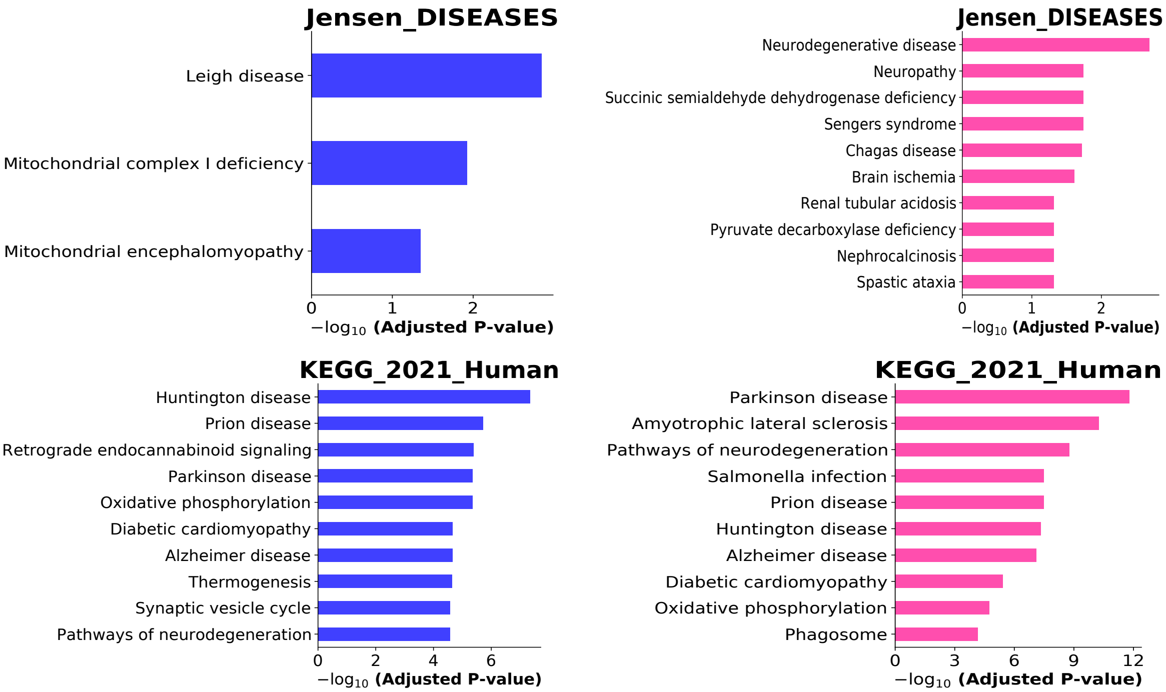


(b)

Figure S11: Disease and pathways associated with temporal cortex using DisGeNET, Jensen and KEGG libraries in proteins rhythmic in control subjects but not AD (blue) and proteins rhythmic in AD subject but not in control (pink).

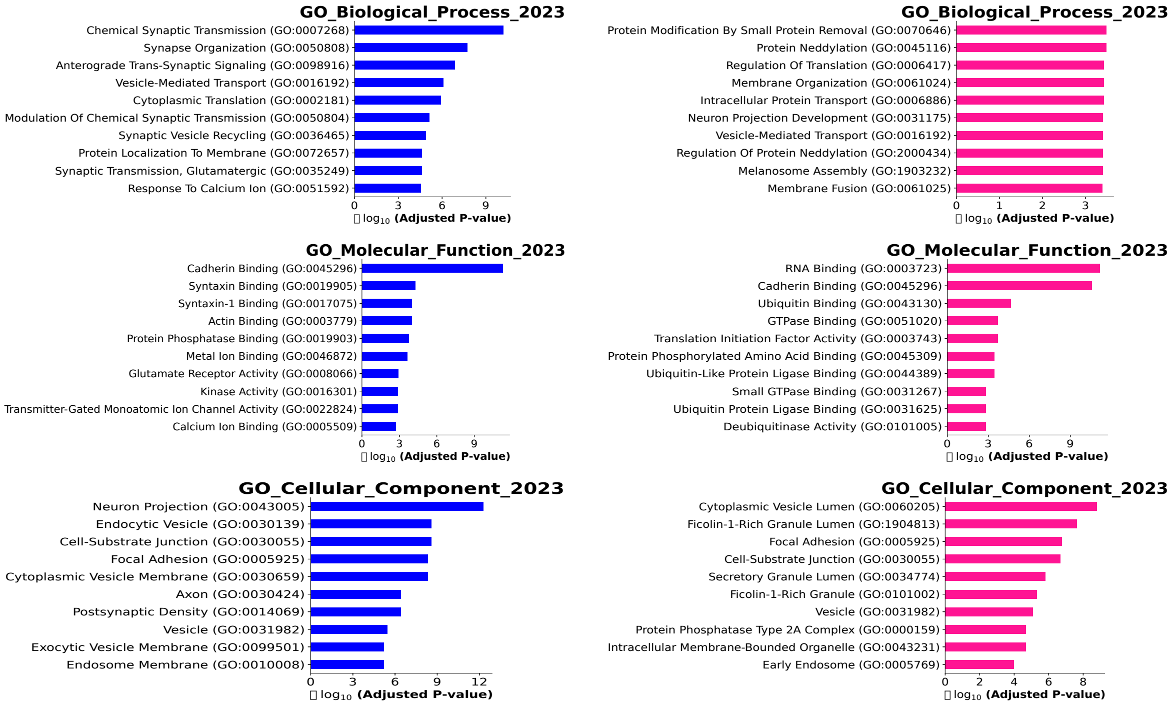


Figure S12: Gene Ontology enrichment analysis of proteins rhythmic in control subjects but not AD (blue) and AD subject but not in control (pink) in parietal association cortex.

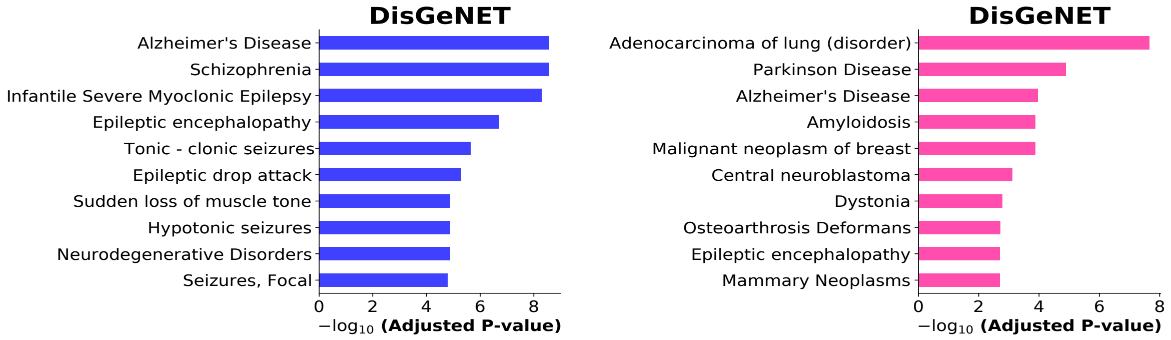


(a)

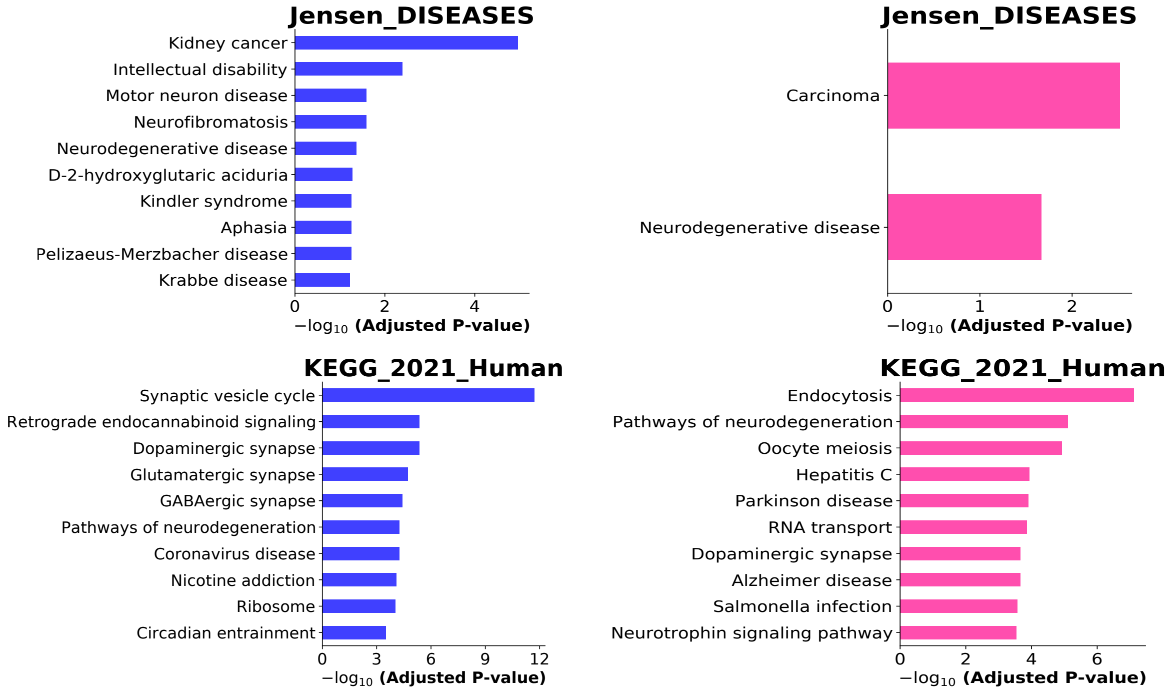


(b)

Figure S13: Disease and pathways associated with parietal association cortex using DisGeNET, Jensen and KEGG libraries in proteins rhythmic in control subjects but not AD (blue) and proteins rhythmic in AD subject but not in control (pink).

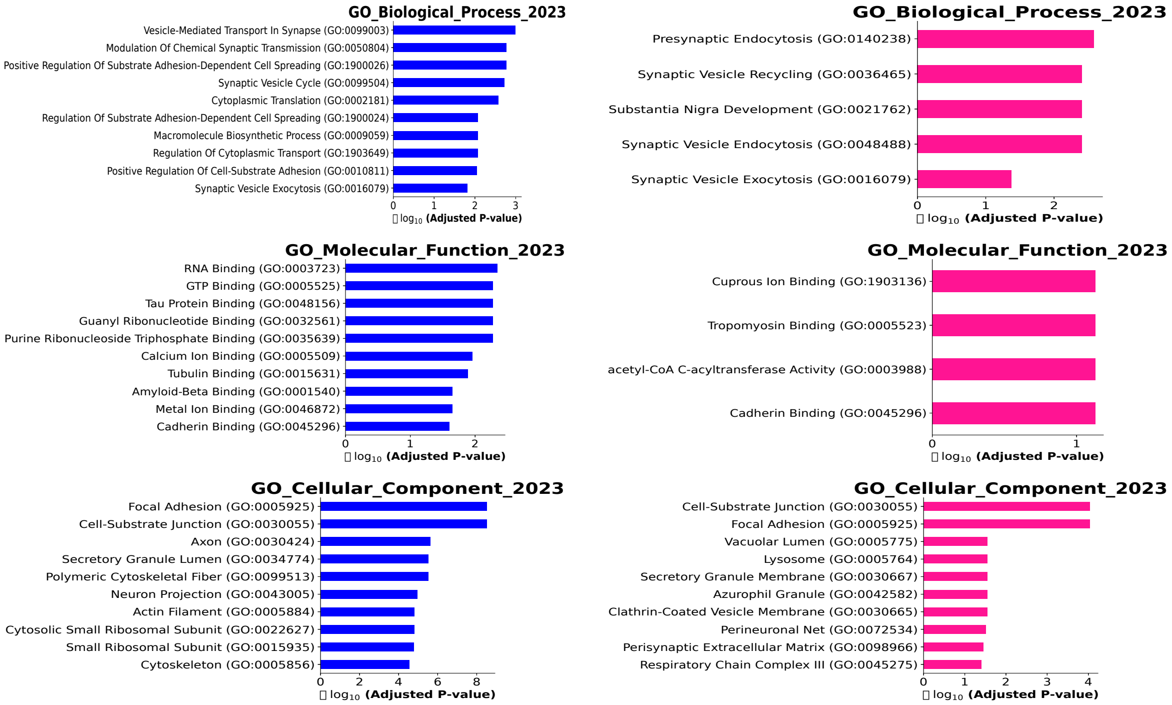


Figure S14: Gene Ontology enrichment analysis of proteins rhythmic in control subjects but not AD (blue) and AD subject but not in control (pink) in DLFPC brain region.

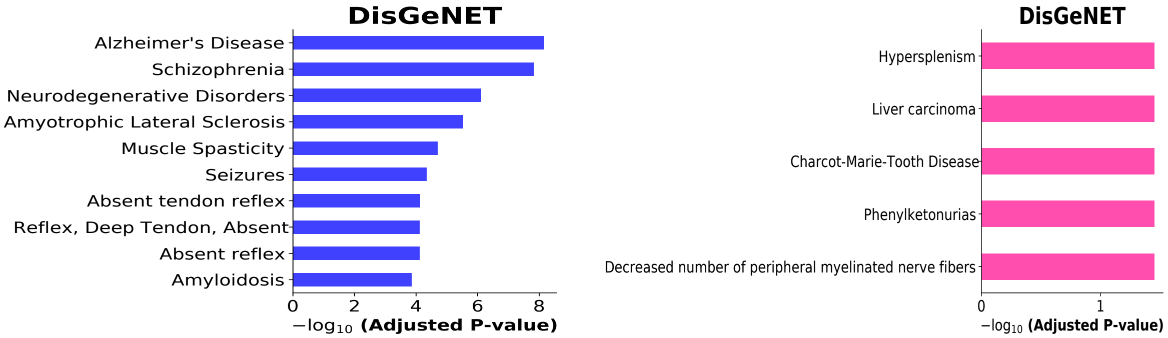


(a)

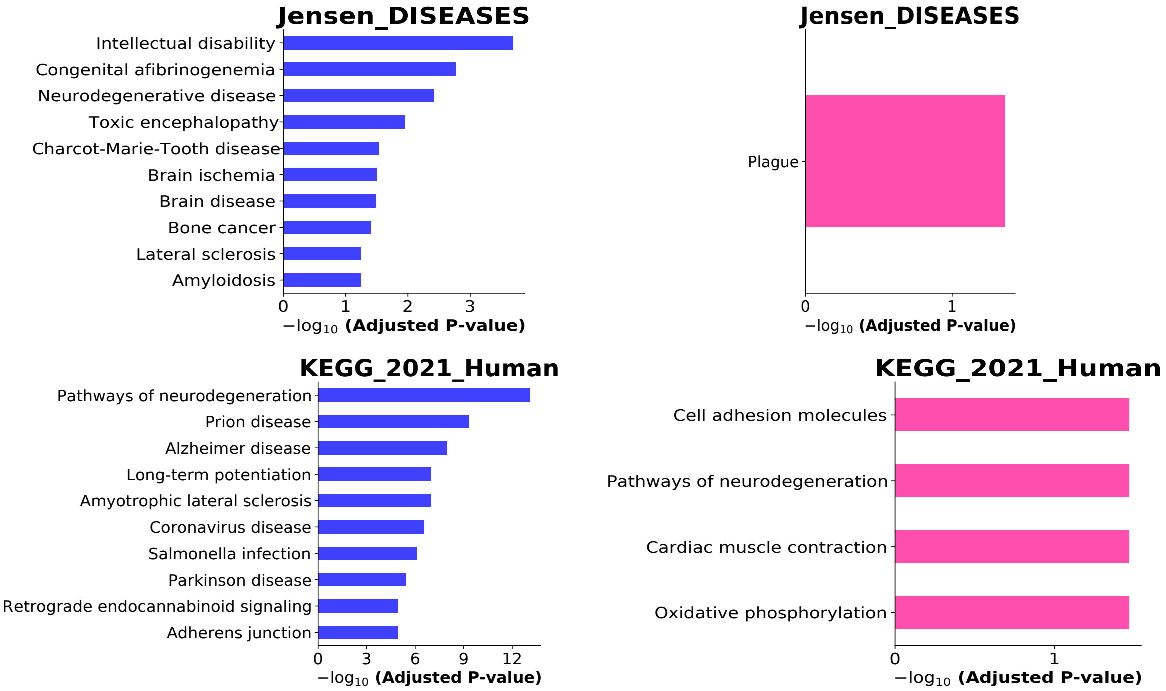


(b)

Figure S15: Disease and pathways associated with DLFPC region using DisGeNET, Jensen and KEGG libraries in proteins rhythmic in control subjects but not AD (blue) and proteins rhythmic in AD subject but not in control (pink).

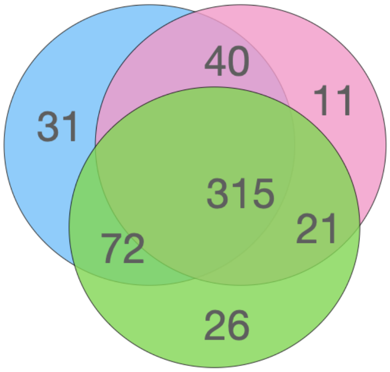


Figure S16: Venn diagram of numbers of rhythmic proteins in control (blue), AD (pink) and MCI (green) subjects in Urine dataset.

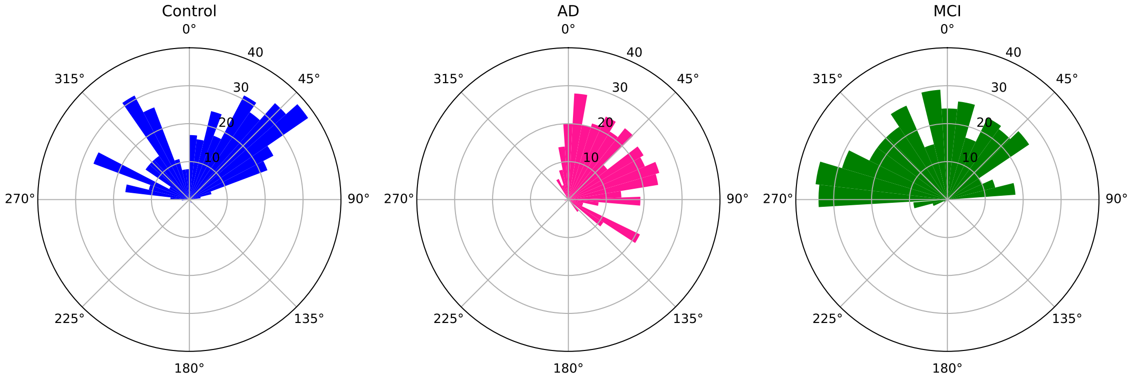


Figure S17: Rose plots of distributions of peak times (i.e., acrophases) in control, AD and MCI subjects in Urine dataset. Each radial distance indicates protein counts.

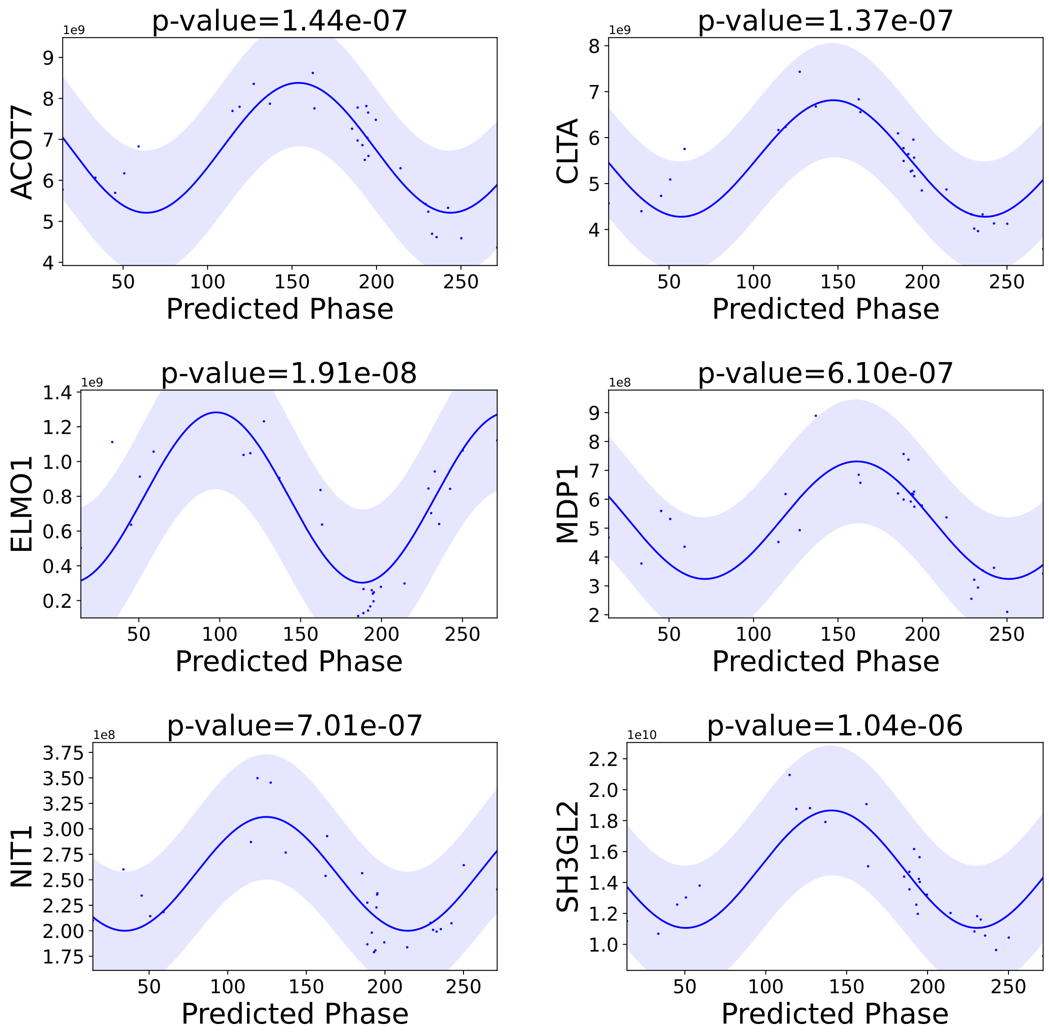


Figure S18: Ultradian proteins found in temporal cortex with period of 12 hours.

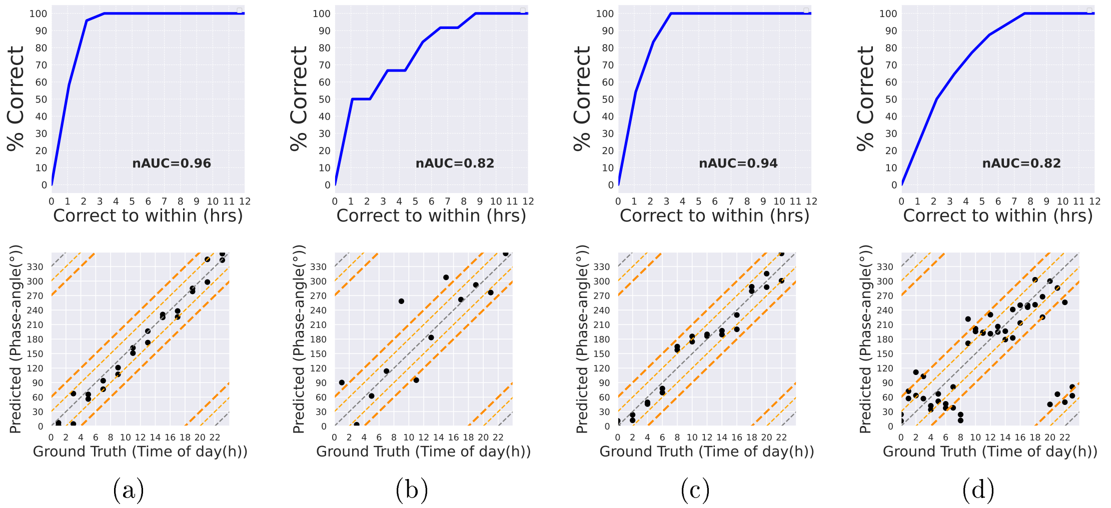


Figure S19: Accuracy of PROTECT on transcriptomic and metabolomic data. (a) mouse liver transcriptomic, (b) baboon amygdala transcriptomic, (c) mouse kidney transcriptomic, and (d) mouse liver metabolomic . The top row shows ROC curves where the y-axis shows the fraction of correctly predicted samples, and the x-axis shows the size of errors. The bottom row shows the scatter plots of predictions vs ground truth.
